# Supplementary material for: Computability and Tiling Problems
Source: arXiv:2307.13075 source file (2023-07-20)
Supplement: Supplementary file 1 [file appendix1.tex]

\addcontentsline{toc}{chapter}{Appendix}

% this is set for multiple appendices. Comment out and use the commented line below if only one Appendix.
\chapter*{Appendices\markboth{Appendices}{}}
%\chapter*{Appendix \markboth{Appendix \thesection}{}}

%\renewcommand{\thesubsection}{\Alph{section}.\arabic{subsection}}

\appendix

%-------------------------------------------------------------------------------

\section{Title of Appendix 1}\label{appendix1}

Insert text here

\clearpage
\newpage
\section{Title of Appendix 2}\label{appendix2}

Insert text here
